# Supplementary material for: Multi-modal Knowledge Distillation-based Human Trajectory Forecasting
Source: arXiv:2503.22201 source file (2025-03-28)
Supplement: Supplementary file 1 [file X_suppl.tex]

\clearpage
\setcounter{page}{1}
\maketitlesupplementary
\section{Overview}
The supplementary material provides further insight to our paper. 
The contents are as follows:\\
% -Section~\ref{supp_sec:clarifications}: Clarifications and corrections on main paper\\
-Section~\ref{supp_sec: model implementation}: Details on model implementation\\
-Section~\ref{supp_sec:dataset}: Details on dataset\\
-Section~\ref{sec_supp:ablations}: Further results and ablations\\
-Section~\ref{sec_supp:qual}: More qualitative results\\
-Section~\ref{sec:limitations}: Limitations\\

% \section{Clarifications and corrections on main paper}
% \label{supp_sec:clarifications}
% We apologize for any confusion due to missing information or misleading notations. 
% We clarify these as follows.
% The main paper will be corrected before publication.
% Thank you for your generous understanding.\\
% - JRDB~\cite{martin2021jrdb} and SIT~\cite{bae2024sit} datasets are parsed with 2.5FPS to predict 12 frames given 8 frames, matching the setting for ETH~\cite{pellegrini2009you}/UCY~\cite{lerner2007crowds} dataset.\\
% - \colorbox{gray!60}{Items with dark background} in the tables of main paper and supplementary materials denote the performances of student model trained with our KD (knowledge distillation) framework.\\
% - The model employing modalities $\mathcal{X}+\mathcal{P}+\mathcal{S}$, as presented in Table 1 of the main paper, serves as the teacher model for both HiVT and MART on the JRDB and SIT datasets. Likewise, the teacher model for the ETH and UCY datasets is also chosen as $\mathcal{X}+\mathcal{P}+\mathcal{S}$.\\
% - Notations $s_\text{R}$, $s_\text{r}$, $\mathcal{S}_\text{R}$ all denote interaction relationship text parsed from the annotation of JRDB dataset. We use notation $\mathcal{S}_\text{R}$ for interaction relationship text in the supplementary materials.\\
% - Both $K, F$ are used as notation for predicted trajectory number of modes. We will standardize the notation as $F$.
% 표 검은 부분
% text 관련
% Teacher model

\section{Details on model implementation}
\label{supp_sec: model implementation}
\subsection{LED}
The denoising process of original LED model is analogous to a latent diffusion model~\cite{rombach2022high}, where the latent encoded from historical information is used for each denoising step.
For both $\mathcal{X}$ and $\mathcal{X}+\mathcal{P}$ models, we add a heading vector (at t=0) embedding encoded from MLP for instantaneous predictions when encoding the latent for denoising.
For $\mathcal{X}+\mathcal{P}$ model, we additionally acquire pose embeddings with MLP followed by cross attention across trajectory and pose embeddings to acquire the final historical latent used for denoising.
Attention across trajectory and pose embeddings for all timesteps and heading vector embedding are holistically considered.
Total number of parameters is 3.6M.
\subsection{socialTransmotion}
Similarly, we add heading vector embedding for both $\mathcal{X}$ and $\mathcal{X}+\mathcal{P}$ models as a additional token to be considered for cross attention.
We preserve all other network designs for both models.
Total number of parameters is 3.9M.
\subsection{MART}
Details are found in the main paper.
Total number of parameters is 3.0M.
\subsection{HiVT}
Details are found in the main paper.
Total number of parameters is 3.3M.

\section{Details on dataset}
\label{supp_sec:dataset}
\subsection{JRDB/SIT dataset}
For both JRDB and SIT datasets, we first extract the global location from 3D bounding box annotations and use them as trajectories for each agent in each frame.
We adjust the FPS to 2.5 frames per second and predict 12 frames given 8 frames to match the setting for ETH/UCY dataset.
Human pose is extracted for agents within a distance $\zeta$ and with no occlusion via SOTA 3D pose estimation algorithm~\cite{sun2022putting}.
The body orientation around the height axis is rotated based on the z-axis rotation angle provided in 3D bounding box annotation.
$\zeta$ is set as 5m for JRDB and 10m for SIT to minimize noise incorporated with human pose.
Single image resolution for JRDB is inferior with 752 $\times$ 480 while SIT image resolution acquired as 1920 $\times$ 1200, allowing for accurate pose acquisition on agents further away for SIT dataset.
For JRDB dataset, text annotation $\mathcal{S}$ includes both agent caption $\mathcal{S}_\text{A}$ describing what the agent is doing and interaction relationship caption $\mathcal{S}_\text{R}$ between certain agents involved in a same activity.
For SIT dataset, no text annotations are provided, so we use vision language model (VLM)~\cite{xu2024pllava} to acquire agent caption $\mathcal{S}_\text{A}$ for each visible agent.
Specifically, we use cropped images around the bounding box for all historical timesteps, therefore a total of 8 frames are used for captioning an agent of a given timestep.
Algorithm~\ref{algorithm:jrdb_sit} describes the process of constructing the JRDB and SIT dataset.

\begin{algorithm}
    \caption{JRDB/SIT dataset construction algorithm}
    \label{JRDBSIT_algorithm}
    \begin{algorithmic}
    % \State $i \gets 10$
    \For{$t = 1$, $t{+}{+}$, while $t < T$}
        % \State{Extract $P_{t,i}^{3D,X}$}
        \State $N \gets \text{number of persons with 3D bounding box}$ \\         $\hspace{4em} \text{annotation}$
        \For{$n = 1$, $n{+}{+}$, while $n <= N$}
            \State $\mathcal{M}_n^t \gets X_n^t$
            \If{$L2(X_{robot}^t, X_n^t) < \zeta$ \textbf{and} No occlusion}
                \State $\mathcal{M}_n^t \gets \phi_{\mathcal{P}}(I_{n}^{t})$
                \If{SIT}
                    \State $\mathcal{M}_n^t \gets \phi_{\mathcal{S}}(\phi_{\mathcal{\text{VLM}}}(I_{n}^{t-T_F:t}))$
                \EndIf
            \EndIf
            \If{JRDB}
                \State $\mathcal{M}_n^t \gets \phi_{\mathcal{S}}(\mathcal{S}_\text{A})$
                \State $\mathcal{M}_n^t \gets \phi_{\mathcal{S}}(\mathcal{S}_\text{R})$
            \EndIf
        \EndFor
    \EndFor
    \end{algorithmic}
    \label{algorithm:jrdb_sit}
\end{algorithm}

In algorithm~\ref{algorithm:jrdb_sit}, $I_n^t$ denotes a cropped image for agent $n$ on timestep $t$, and $\mathcal{M}_n^t$ denotes modality information available for agent $n$ on timestep $t$. 
Also, while only agent description caption $\mathcal{S}_\text{A}$ is acquired for SIT dataset, we additionally utilize agent relationship caption $\mathcal{S}_\text{R}$ from annotations for JRDB dataset.
$\phi_{\mathcal{P}}$ denotes pose extractor~\cite{sun2022putting}, $\phi_{\mathcal{S}}$ denotes pre-trained BERT encoder~\cite{devlin2018bert}, and $\phi_{\text{VLM}}$ denotes vision-language model (VLM)~\cite{xu2024pllava} used to acquire caption for each agent.
While the default prompt to acquire caption is set as "What is the person doing?", we also compare using different prompts as shown in table 6 of main paper.

The exact prompts used are as follows:\\
\textbf{Prompt 1}\\
Shortened: "what is the person doing?"\\
Full: "The input consists of camera view from a mobile robot. In the images, people are standing still or walking, alone or in a group. Your job is to describe the behavior of the person marked with red bounding box. What is the person doing? In one full sentence. Concisely, less than 20 words. Do not talk about clothing of person."\\
\textbf{Prompt 2}\\
Shortened: "Is there any obstacle in front of the person?"\\
Full: "The input consists of camera view from a mobile robot. In the images, people are standing still or walking, alone or in a group. Is there any obstacle in the way of person with red bounding box? In one full sentence. Concisely, less than 20 words."\\
\textbf{Prompt 3}\\
Shortened: "What will the person do in the future?"\\
Full: "The input consists of camera view from a mobile robot. In the images, people are standing still or walking, alone or in a group. What will the person in red bounding box do in the future? In one full sentence. Concisely, less than 20 words."

\begin{figure*}
    \includegraphics[width=0.99\textwidth]{figures_supp/sit_prompt.PNG} \vspace{-7pt}
    \caption{
    Examples of images used for captioning via VLM and the acquired agent captions $\mathcal{S}_\text{A}$ for SIT dataset. 
    Colors denote the type of prompts used on the VLM.
    Each image denotes the last frame of 8 frames used for captioning.
    Person of interest is marked by the red bounding box.
    }
    \label{fig:sit_prompt}
    \vspace{-5pt}
\end{figure*}

Figure~\ref{fig:sit_prompt} compares the acquired agent captions $\mathcal{S}_\text{A}$ with different prompts.

\subsection{ETH/UCY dataset}
While overall dataset construction process for ETH/UCY is analogous to that of JRDB/SIT, the main difference is the form of representation for pose and how text captions are obtained.
For human pose, we use 2D CLIP vision encoder~\cite{radford2021learning} features instead of 3D pose, as an accurate 3D pose was unable to be obtained due to the low resolution and limited visibility of BEV (Bird eye view) perspective.
For text, neither agent-specific captions are available or VLM able to obtain text captions.
Specifically, as VLM failed to generate accurate captions with a low resolution BEV input, we resort to a rule-based method to generate text captions that captures the surrounding obstacle information for each agent.
In doing so, we use 2D walkable area segmentation map in image coordinates to generate text captions that contain map information for each agent.
Text is generated based on agent's speed and surrounding obstacles.
The following algorithm is used to construct the dataset.

\begin{algorithm}
    \caption{ETH/UCY dataset construction algorithm}
    \label{ETHUCY_algorithm}
    \begin{algorithmic}
    % \State $i \gets 10$
    \For{$t = 1$, $t{+}{+}$, while $t < T$}
        % \State{Extract $P_{t,i}^{3D,X}$}
        \State $N \gets \text{number of persons with location annotation}$
        \For{$n = 1$, $n{+}{+}$, while $n <= N$}
            \State $\mathcal{M}_n^t \gets X_n^t$
            \State $\mathcal{M}_n^t \gets \phi_{\mathcal{P}}(I_{n}^{t})$
            \State $\mathcal{S}_n^t=\text{` '}$
            \If{$L2(X_n^t, X_n^{t-1}) < 1.5 \text{pixels}$}
                \State $\mathcal{S}_n^t \gets \text{`The person is standing still.'}$
            \ElsIf{$L2(X_n^t, X_n^{t-1}) < 20 \text{pixels}$}
                \State $\mathcal{S}_n^t \gets \text{`The person is walking slowly.'}$
            \Else
                \State $\mathcal{S}_n^t \gets \text{`The person is walking.'}$
            \EndIf
            
            \If{$L2(\text{Nearest obstacle}, X_n^t) < \zeta$}
                \State $\sigma=\text{Heading vector} - \text{Obstacle vector}$
                \If{$\sigma > 30^\circ$ and $\sigma < 100^\circ$}
                    \State $\mathcal{S}_n^t \gets \text{`There is an obstacle on the right.'}$
                \ElsIf{$\sigma < 30^\circ$ and $\sigma > -30^\circ$}
                    \State $\mathcal{S}_n^t \gets \text{`There is an obstacle in front.'}$
                \ElsIf{$\sigma < -30^\circ$ and $\sigma > -100^\circ$}
                    \State $\mathcal{S}_n^t \gets \text{`There is an obstacle on the left.'}$
                \Else
                    \State $\mathcal{S}_n^t \gets \text{`There is no obstacle in the heading}$ \\         $\hspace{4em} \text{direction of the person.'}$
                \EndIf
            \Else
                \State $\mathcal{S}_n^t \gets \text{`There is no obstacle around.'}$
            \EndIf
            \State $\mathcal{M}_n^t \gets \phi_\mathcal{S}(\mathcal{S}_n^t)$
        \EndFor
    \EndFor
    \end{algorithmic}
\end{algorithm}

In algorithm~\ref{ETHUCY_algorithm}, heading vector is the vector from $X_n^{t-1}$ to $X_n^t$, which is same as the heading vector used for rotation-invariant encoding of HiVT~\cite{zhou2022hivt}.
Obstacle vector is vector from $X_n^t$ to the point of closest obstacle. 

\subsection{Dataset visualization}
Figures~\ref{fig:jrdbViz1}, \ref{fig:jrdbViz2} visualize two scenes from JRDB dataset, one from indoor and one from outdoor. 
For JRDB scenes, we show agent and interaction text captions for only a few selected agents for compact visualization.
For SIT dataset visualized in Fig.~\ref{fig:sitViz}, the captions are acquired with the default prompt ``What is the person doing?''.
Origin denotes position of robot which captured the scene with omnidirectional cameras.

\subsection{Scene parsing for Train/Validation sets}
As only training sets of JRDB/SIT are provided with full annotations (3D bounding box, 2D bounding box, text annotation), we parse the training set of the initially provided dataset into train (85\%) and validation sets (15\%).
The parsed validation set contains a similar ratio of indoor and outdoor scenes.\\
Scenes for JRDB train set parsing: 
\begin{itemize}[nosep]
    \item \texttt{clark-center-2019-02-28\_0}
    \item \texttt{clark-center-2019-02-28\_1}
    \item \texttt{clark-center-intersection-2019-02-28\_0}
    \item \texttt{cubberly-auditorium-2019-04-22\_0}
    \item \texttt{forbes-cafe-2019-01-22\_0}
    \item \texttt{gates-159-group-meeting-2019-04-03\_0}
    \item \texttt{gates-ai-lab-2019-02-08\_0}
    \item \texttt{gates-basement-elevators-2019-01-17\_1}
    \item \texttt{hewlett-packard-intersection-2019-01-24\_0}
    \item \texttt{huang-2-2019-01-25\_0}
    \item \texttt{huang-basement-2019-01-25\_0}
    \item \texttt{gates-to-clark-2019-02-28\_1}
    \item \texttt{memorial-court-2019-03-16\_0}
    \item \texttt{meyer-green-2019-03-16\_0}
    \item \texttt{nvidia-aud-2019-04-18\_0}
    \item \texttt{packard-poster-session-2019-03-20\_1}
    \item \texttt{packard-poster-session-2019-03-20\_2}
    \item \texttt{stlc-111-2019-04-19\_0}
    \item \texttt{svl-meeting-gates-2-2019-04-08\_0}
    \item \texttt{svl-meeting-gates-2-2019-04-08\_1}
    \item \texttt{tressider-2019-03-16\_0}
    \item \texttt{tressider-2019-03-16\_1}
    \item \texttt{tressider-2019-03-16\_2}
\end{itemize}

Scenes for JRDB validation set parsing: 
\begin{itemize}[nosep]
    \item \texttt{bytes-cafe-2019-02-07\_0}
    \item \texttt{huang-lane-2019-02-12\_0}
    \item \texttt{jordan-hall-2019-04-22\_0}
    \item \texttt{packard-poster-session-2019-03-20\_0}
\end{itemize}

Scenes for SIT train set parsing: 
\begin{itemize}[nosep]
    \item \texttt{Cafe\_street\_2-001}
    \item \texttt{Cafeteria\_1-006}
    \item \texttt{Cafeteria\_2-005}
    \item \texttt{Cafeteria\_5-003}
    \item \texttt{Corridor\_2-007}
    \item \texttt{Corridor\_3-004}
    \item \texttt{Corridor\_5-003}
    \item \texttt{Corridor\_7-001}
    \item \texttt{Corridor\_8-006}
    \item \texttt{Corridor\_9-011}
    \item \texttt{Corridor\_10-009}
    \item \texttt{Corridor\_11-002}
    \item \texttt{Courtyard\_1-009}
    \item \texttt{Courtyard\_2-002}
    \item \texttt{Courtyard\_4-008}
    \item \texttt{Courtyard\_5-005}
    \item \texttt{Courtyard\_6-007}
    \item \texttt{Courtyard\_8-001}
    \item \texttt{Courtyard\_9-003}
    \item \texttt{Crossroad\_1-001}
    \item \texttt{Hallway\_1-011}
    \item \texttt{Hallway\_2-003}
    \item \texttt{Hallway\_3-001}
    \item \texttt{Hallway\_4-012}
    \item \texttt{Hallway\_6-009}
    \item \texttt{Hallway\_7-010}
    \item \texttt{Hallway\_8-005}
    \item \texttt{Hallway\_9-008}
    \item \texttt{Hallway\_10-006}
    \item \texttt{Hallway\_11-002}
    \item \texttt{Lobby\_2-009}
    \item \texttt{Lobby\_3-007}
    \item \texttt{Lobby\_4-002}
    \item \texttt{Lobby\_5-008}
    \item \texttt{Lobby\_7-004}
    \item \texttt{Lobby\_8-003}
    \item \texttt{Outdoor\_Alley\_2-003}
    \item \texttt{Subway\_Entrance\_2-004}
    \item \texttt{Subway\_Entrance\_4-003}
    \item \texttt{Three\_way\_Intersection\_3-006}
    \item \texttt{Three\_way\_Intersection\_4-001}
    \item \texttt{Three\_way\_Intersection\_5-005}
    \item \texttt{Three\_way\_Intersection\_8-002}
\end{itemize}

Scenes for SIT validation set parsing: 
\begin{itemize}[nosep]
    \item \texttt{Cafe\_street\_1-002}
    \item \texttt{Cafeteria\_3-004}
    \item \texttt{Corridor\_1-010}
    \item \texttt{Lobby\_6-001}
    \item \texttt{Outdoor\_Alley\_3-002}
    \item \texttt{Three\_way\_Intersection\_4-001}
    \item \texttt{Subway\_Entrance\_2-004}
\end{itemize}

Furthermore, Tab.~\ref{tab:dataset_comparison} compares the statistics between JRDB and SIT dataset.
JRDB dataset consists of more complex scenes with larger average and maximum number of agents in a given sequence.
In addition, total duration of JRDB is 2$\times$ than SIT dataset, making JRDB a more challenging and thorough dataset.

\begin{table}[]
\centering
\caption{Statistical comparison between JRDB and SIT datasets.}
\resizebox{\columnwidth}{!}{%
\begin{tabular}{|c|c|c|c|c|c|c|}
\hline
     & Duration (s) & Indoor \# & Outdoor \# & Sample \# & Max $N$ & Avg. $N$\\ \hline
JRDB & 1860         & 17        & 10         & 24788     & 38                                                       & 16                                                       \\ \hline
SIT  & 940          & 4         & 6          & 5141      & 19                                                       & 6                                                        \\ \hline
\end{tabular}%
}
\label{tab:dataset_comparison}
\end{table}

\begin{table*}[]
\caption{Prediction results on ETH/UCY (Average) with different modality ($\mathcal{M}$) combinations, with human pose ($\mathcal{M}$) and text ($\mathcal{S}$) as additional input. Trained with all regression losses ($\mathcal{L}_\text{reg}^\text{F}$,$\mathcal{L}_\text{reg}^\text{2}$,$\mathcal{L}_\text{reg}^\text{1}$). Bold denotes best. Lower is better.}
\vspace{-7pt}
\resizebox{\textwidth}{!}{
\begin{tabular}{|c|ccccccc|ccccccc|}
\hline
\multirow{2}{*}{$\mathcal{M}$} & \multicolumn{7}{c|}{HiVT} & \multicolumn{7}{c|}{MART} \\ \cline{2-15} 
 & ADE & \text{ADE}\textsubscript{2} & \text{ADE}\textsubscript{1} & FDE & \text{FDE}\textsubscript{2} & \multicolumn{1}{c|}{\text{FDE}\textsubscript{1}} & Avg. +\% & ADE & \text{ADE}\textsubscript{2} & \text{ADE}\textsubscript{1} & FDE & \text{FDE}\textsubscript{2} & \multicolumn{1}{c|}{\text{FDE}\textsubscript{1}} & Avg. +\% \\ \hline
$\mathcal{X}$ & \textbf{0.314} & \textbf{0.320} & 0.555 & \textbf{0.718} & \textbf{0.726} & \multicolumn{1}{c|}{1.132} & - & 0.364 & 0.369 & 0.571 & 0.852 & 0.862 & \multicolumn{1}{c|}{1.166} & - \\
$\mathcal{X}+\mathcal{S}$ & 0.331 & 0.340 & 0.490 & 0.748 & 0.760 & \multicolumn{1}{c|}{1.005} & +0.45 & 0.355 & \textbf{0.360} & 0.521 & \textbf{0.823} & \textbf{0.828} & \multicolumn{1}{c|}{1.083} & +4.69 \\
$\mathcal{X}+\mathcal{P}+\mathcal{S}$ & 0.339 & 0.350 & \textbf{0.444} & 0.761 & 0.772 & \multicolumn{1}{c|}{\textbf{0.920}} & \textbf{+1.57} & \textbf{0.352} & 0.367 & \textbf{0.472} & 0.852 & 0.871 & \multicolumn{1}{c|}{\textbf{1.064}} & \textbf{+4.81} \\ \hline
\end{tabular}
}
\label{table:ethucy_multimodal}
\end{table*}

\begin{table*}[]
\caption{Prediction results on JRDB with different modality ($\mathcal{M}$) combinations, with human pose ($\mathcal{M}$) and text ($\mathcal{S}$) as additional input. Only trained on regression loss with full past observation, $\mathcal{L}_\text{reg}^\text{F}$. Bold denotes best. Lower is better.}
\vspace{-7pt}
\resizebox{\textwidth}{!}{
\begin{tabular}{|c|ccccccc|ccccccc|}
\hline
\multirow{2}{*}{$\mathcal{M}$} & \multicolumn{7}{c|}{HiVT} & \multicolumn{7}{c|}{MART} \\ \cline{2-15} 
 & ADE & \text{ADE}\textsubscript{2} & \text{ADE}\textsubscript{1} & FDE & \text{FDE}\textsubscript{2} & \multicolumn{1}{c|}{\text{FDE}\textsubscript{1}} & Avg. +\% & ADE & \text{ADE}\textsubscript{2} & \text{ADE}\textsubscript{1} & FDE & \text{FDE}\textsubscript{2} & \multicolumn{1}{c|}{\text{FDE}\textsubscript{1}} & Avg. +\% \\ \hline
$\mathcal{X}$ & 0.223 & 0.246 & 0.718 & 0.434 & 0.476 & \multicolumn{1}{c|}{1.231} & - & 0.274 & 0.288 & 0.629 & 0.526 & 0.547 & \multicolumn{1}{c|}{1.127} & - \\
$\mathcal{X}+\mathcal{P}$ & 0.229 & 0.251 & 0.573 & 0.448 & 0.486 & \multicolumn{1}{c|}{1.015} & +4.65 & 0.291 & 0.294 & 0.596 & 0.549 & 0.551 & \multicolumn{1}{c|}{1.097} & -0.90 \\
$\mathcal{X}+\mathcal{S}$ & \textbf{0.220} & \textbf{0.240} & 0.449 & \textbf{0.430} & \textbf{0.462} & \multicolumn{1}{c|}{0.848} & +12.72 & \textbf{0.267} & \textbf{0.265} & \textbf{0.347} & \textbf{0.517} & 0.513 & \multicolumn{1}{c|}{\textbf{0.643}} & \textbf{+17.75} \\
$\mathcal{X}+\mathcal{P}+\mathcal{S}$ & 0.223 & 0.242 & \textbf{0.437} & 0.438 & 0.469 & \multicolumn{1}{c|}{\textbf{0.782}} & \textbf{+12.98} & 0.278 & 0.270 & 0.403 & 0.528 & \textbf{0.512} & \multicolumn{1}{c|}{0.721} & +13.79 \\ \hline
\end{tabular}
}
\label{table:supp_onlyFullTimestep}
\end{table*}

\begin{table}[]
\caption{Ablation on representation format for pose $\mathcal{P}$. Exprimented on JRDB dataset with HiVT $\mathcal{X}+\mathcal{P}$ model.}
\resizebox{\columnwidth}{!}{%
\begin{tabular}{|c|c|c|cccccc|c|}
\hline
Model & \cellcolor[HTML]{FFFFFF}$\mathcal{P}$ type & \cellcolor[HTML]{FFFFFF}\begin{tabular}[c]{@{}c@{}}w/ \\ KD\end{tabular} & ADE & \text{ADE}\textsubscript{2} & \text{ADE}\textsubscript{1} & FDE & \text{FDE}\textsubscript{2} & \text{FDE}\textsubscript{1} & \begin{tabular}[c]{@{}c@{}}Avg. \\ +\%\end{tabular} \\ \hline
 &  &  & 0.288 & 0.286 & 0.394 & 0.553 & 0.547 & 0.727 & \multicolumn{1}{l|}{} \\
 & \multirow{-2}{*}{3D joint} & \checkmark & 0.271 & 0.268 & 0.381 & 0.520 & 0.517 & 0.721 & - \\ \cline{2-10} 
 &  &  & \textbf{0.287} & \textbf{0.282} & \textbf{0.366} & \textbf{0.543} & \textbf{0.538} & \textbf{0.682} & +3.08 \\
\multirow{-4}{*}{MART} & \multirow{-2}{*}{SMPL} & \cellcolor[HTML]{DADADA}\checkmark & \cellcolor[HTML]{DADADA}\textbf{0.266} & \cellcolor[HTML]{DADADA}\textbf{0.261} & \cellcolor[HTML]{DADADA}\textbf{0.337} & \cellcolor[HTML]{DADADA}\textbf{0.519} & \cellcolor[HTML]{DADADA}\textbf{0.507} & \cellcolor[HTML]{DADADA}\textbf{0.633} & \textbf{+5.07} \\ \hline
 &  &  & 0.232 & 0.248 & \textbf{0.354} & 0.446 & 0.480 & \textbf{0.646} & - \\
 & \multirow{-2}{*}{3D joint} & \checkmark & \textbf{0.229} & 0.240 & 0.325 & 0.446 & 0.464 & 0.598 & - \\ \cline{2-10} 
 &  &  & \textbf{0.229} & \textbf{0.242} & 0.364 & \textbf{0.441} & \textbf{0.465} & 0.659 & +0.56 \\
\multirow{-4}{*}{HiVT} & \multirow{-2}{*}{SMPL} & \cellcolor[HTML]{DADADA}\checkmark & \cellcolor[HTML]{DADADA}0.232 & \cellcolor[HTML]{DADADA}\textbf{0.239} & \cellcolor[HTML]{DADADA}\textbf{0.308} & \cellcolor[HTML]{DADADA}\textbf{0.445} & \cellcolor[HTML]{DADADA}\textbf{0.464} & \cellcolor[HTML]{DADADA}\textbf{0.560} & \textbf{+1.87} \\ \hline
\end{tabular}
} 
\label{table:smpl_joint}
\end{table}

\begin{table}[]
\caption{Ablation on using different combinations for regression loss ($\mathcal{L}_\text{reg}^\text{F}$, $\mathcal{L}_\text{reg}^\text{1}$, $\mathcal{L}_\text{reg}^\text{2}$) on student, teacher models. Experimented on JRDB.}
\vspace{-7pt}
\resizebox{\columnwidth}{!}{%
\begin{tabular}{|cc|cc|cccccc|}
\hline
\multicolumn{2}{|c|}{Teacher} & \multicolumn{2}{c|}{Student} & \multicolumn{6}{c|}{Metrics} \\ \hline
$\mathcal{L}^\text{F}_\text{reg}$ &$\mathcal{L}^\text{2,1}_\text{reg}$ & $\mathcal{L}^\text{F}_\text{reg}$ &$\mathcal{L}^\text{2,1}_\text{reg}$ & ADE & \multicolumn{1}{l}{\text{ADE}\textsubscript{2}} & \text{ADE}\textsubscript{1} & FDE & \multicolumn{1}{l}{\text{FDE}\textsubscript{2}} & \text{FDE}\textsubscript{1}\\ \hline
\checkmark & \multicolumn{1}{l|}{} & \checkmark & \multicolumn{1}{l|}{} & 0.227 & 0.282 & 0.725 & 0.442 & 0.546 & 1.330 \\
\checkmark & \checkmark & \checkmark & \multicolumn{1}{l|}{} & \textbf{0.222} & \textbf{0.277} & \textbf{0.498} & \textbf{0.431} & \textbf{0.534} & \textbf{0.907} \\ \hline
\checkmark & \multicolumn{1}{l|}{} & \checkmark & \checkmark & \textbf{0.222} & \textbf{0.233} & 0.319 & \textbf{0.437} & \textbf{0.452} & 0.578 \\
\cellcolor[HTML]{DADADA}\checkmark & \cellcolor[HTML]{DADADA}\checkmark & \cellcolor[HTML]{DADADA}\checkmark & \cellcolor[HTML]{DADADA}\checkmark & \cellcolor[HTML]{DADADA}0.232 & \cellcolor[HTML]{DADADA}0.239 &\cellcolor[HTML]{DADADA}\textbf{0.308} &\cellcolor[HTML]{DADADA} 0.445 &\cellcolor[HTML]{DADADA} 0.464 &\cellcolor[HTML]{DADADA} \textbf{0.560} \\ \hline
\end{tabular}
}
\label{table:combination}
\end{table}

\begin{table}[]
\caption{Ablation on number of modes $F$ for KD. Experimented on JRDB with $\mathcal{X}+\mathcal{P}$ HiVT model.}
\vspace{-7pt}
\resizebox{\columnwidth}{!}{%
\begin{tabular}{|c|c|cccccc|c|}
\hline
$F$ & w/ KD & ADE & \text{ADE}\textsubscript{2} & \text{ADE}\textsubscript{1} & FDE & \text{FDE}\textsubscript{2} & \text{FDE}\textsubscript{1} & Avg. +\% \\ \hline
 & \multicolumn{1}{l|}{} & \textbf{0.381} & 0.403 & 0.764 & \textbf{0.729} & 0.772 & 1.341 &  \\
\multirow{-2}{*}{1} & \checkmark & \textbf{0.381} & \textbf{0.389} & \textbf{0.737} & \textbf{0.729} & \textbf{0.757} & \textbf{1.324} & \multirow{-2}{*}{+1.70} \\ \hline
 & \multicolumn{1}{l|}{} & \cellcolor[HTML]{FFFFFF}\textbf{0.229} & \cellcolor[HTML]{FFFFFF}0.242 & \cellcolor[HTML]{FFFFFF}0.364 & \cellcolor[HTML]{FFFFFF}\textbf{0.441} & \cellcolor[HTML]{FFFFFF}0.465 & \cellcolor[HTML]{FFFFFF}0.659 &  \\
\multirow{-2}{*}{6} & \cellcolor[HTML]{DADADA}\checkmark & \cellcolor[HTML]{DADADA}0.232 & \cellcolor[HTML]{DADADA}\textbf{0.239} & \cellcolor[HTML]{DADADA}\textbf{0.308} & \cellcolor[HTML]{DADADA}0.445 & \cellcolor[HTML]{DADADA}\textbf{0.464} & \cellcolor[HTML]{DADADA}\textbf{0.560} & \multirow{-2}{*}{+4.98} \\ \hline
 & \multicolumn{1}{l|}{} & \textbf{0.196} & 0.203 & 0.280 & 0.389 & 0.401 & 0.525 &  \\
\multirow{-2}{*}{10} & \checkmark & \textbf{0.196} & \textbf{0.201} & \textbf{0.273} & \textbf{0.386} & \textbf{0.397} & \textbf{0.505} & \multirow{-2}{*}{+1.56} \\ \hline
 & \multicolumn{1}{l|}{} & 0.160 & 0.165 & 0.235 & 0.314 & 0.322 & 0.428 &  \\
\multirow{-2}{*}{20} & \checkmark & \textbf{0.157} & \textbf{0.163} & \textbf{0.223} & \textbf{0.307} & \textbf{0.321} & \textbf{0.415} & \multirow{-2}{*}{+2.42} \\ \hline
\end{tabular}
}
\label{tab:num_mode}
\end{table}

\section{Further results and ablations}
\label{sec_supp:ablations}
\subsection{Multi-modal teacher model on ETH/UCY}
Table~\ref{table:ethucy_multimodal} highlights the performance enhancements achieved by incorporating additional modalities on the ETH/UCY dataset. Since pose is extracted from cropped images, its generalizability across various scenes is limited. Similar to the JRDB/SIT datasets, text has proven to be the most impactful modality, even when generated using a rule-based approach. These additional modalities are particularly beneficial for instantaneous predictions. Although the absolute percentage improvement is smaller than that observed in the JRDB/SIT datasets due to the limited richness of available modalities, the teacher model leveraging all modalities still outperforms the base model $\mathcal{X}$, indicating potential for further gains through KD.

\subsection{Can we raise a competent teacher while training only on full observation regression?}
In addition to training on all observation settings with $\mathcal{L}_\text{reg}^\text{F}, \mathcal{L}_\text{reg}^\text{2}, \mathcal{L}_\text{reg}^\text{1}$ as shown in table 1 of main paper, we experiment only training with full observation $\mathcal{L}_\text{reg}^\text{F}$.
As shown in Tab.~\ref{table:supp_onlyFullTimestep}, using additional modalities improved the prediction performance even when only trained with $\mathcal{L}_\text{reg}^\text{F}$.
Again, text has been the most crucial modality. 
When only trained on $\mathcal{L}_\text{reg}^\text{F}$ with sufficient past trajectory information, the generalizable nature of text is most valued.
Interestingly, compared to ($\mathcal{X}+\mathcal{P}+\mathcal{S}$) improving over ($\mathcal{X}+\mathcal{S}$) when trained also on $\mathcal{L}_\text{reg}^\text{2,1}$ as shown in main paper table 1, Tab.~\ref{table:supp_onlyFullTimestep} does not show such improvement.
This shows that eliciting a deeper understanding on human intent with pose is most effectively done by training the model on both full ($\mathcal{L}_\text{reg}^\text{F}$) and instantaneous predictions ($\mathcal{L}_\text{reg}^\text{2,1}$), therefore building a more competent teacher model.

\subsection{Which representation of human pose is most effective?}
Table~\ref{table:smpl_joint} compares the prediction performance of HiVT $\mathcal{X}+\mathcal{P}$ model with SMPL theta or 3D joint representations.
For both MART and HiVT, using SMPL as the pose representation leads to improvements in performance, whether or not KD is applied.
The angle-based representation of SMPL clearly captures the inter-joint relationships, making it more resilient to noise and more generalizable compared to the 3D joint representation, where these relationships are not explicitly defined.
In particular, a more significant improvement is seen in models with KD, highlighting that a general angle-based representation can effectively integrate the diverse knowledge from textual descriptions.

\subsection{Can we teach instantaneous prediction without explicit loss during KD?}
Table~\ref{table:combination} presents a comparison of the regression loss combinations used for training the teacher model and the student model during KD. 
The upper two rows compare using different teacher models: teacher additionally trained on instantaneous prediction or only trained on full observation. 
Then, the student model is distilled with regression loss based only on full observation. 
The performance of instantaneous prediction improves significantly when distilled using a teacher model trained on instantaneous predictions. 
This indicates that the teacher’s knowledge of human intent through instantaneous observations is transferable, even without explicit instantaneous loss for the student model. 
Furthermore, when the student model is also trained with $\mathcal{L}_\text{reg}^\text{2,1}$, the student's performance in instantaneous prediction again improves when distilled by a teacher model also trained on instantaneous predictions. 
This once more supports the idea that training on instantaneous predictions fosters a deeper understanding of human motion intent, and that this knowledge is transferable through distillation.

\subsection{Does number of modes have an influence on KD performance?}
Table~\ref{tab:num_mode} compares the KD performance on different number of modes of future trajectory forecasting.
KD consistently enhances the performance of the student model, demonstrating that the knowledge of human motion intent is transferable, regardless of the $F$ configuration used to decode the locomotion intent into multiple trajectories.
This also shows winner-takes-all regression training approach on multiple predictions is effective in transferring knowledge on human motion intent.

\section{More qualitative results}
\label{sec_supp:qual}
Figure~\ref{fig:qualJRDB} visualizes the effect of KD (left two figures) and the effect of using interaction relationship text $\mathcal{S}_\text{R}$ on JRDB dataset.
For KD comparison, the model originally predicts a collision with nearby agents. 
After KD from $\mathcal{X}+\mathcal{P}+\mathcal{S}$ model, the student model predicts a trajectory that avoids collision with other agents, even with only one or two frames of historical observation.
This capability is developed by training the student model leveraging the teacher's extensive knowledge of human motion intent across multiple modalities.

Analysis of interaction relation caption is performed on the rightmost scene of Fig.~\ref{fig:qualJRDB} where two agents are waiting in line, having a conversation, and then walking together.
Without utilizing relationship context, the group dynamic between these two agents is not explicitly accounted for, leading to diverging trajectories. 
In contrast, when the relationship is considered, the two agents initially walk together, and then the front agent moves ahead as the agent is in front in line.
Interestingly, prediction on the agent behind these two agents explicitly described an interaction also improves when using interaction text.
As the model predicts these two agents to walk together, the agent behind them follows the general locomotion flow made by the two agents, resulting in an improved prediction.

Figure~\ref{fig:qualSIT} visualizes the improvement with KD on SIT dataset.
The figure shows a crowded indoor scene with multiple agents in motion.
Predictions made with KD improves upon student without KD for all agents.
Again, using a $\mathcal{X}+\mathcal{P}+\mathcal{S}$ model as a teacher for a $\mathcal{X}+\mathcal{P}$ student enhanced the understanding of locomotion intentions in complex scenes from the comprehensive knowledge gained by the complementary modalities.

\section{Limitations}
\label{sec:limitations}

Our study highlights the potential of incorporating textual information—an effective modality for representing human motion, accessible through Vision-Language Models (VLM)—into trajectory forecasting. This approach allows for a more comprehensive utilization of human pose and trajectory data to understand an agent's locomotion intent. As demonstrated, language can capture not only the intent inferred from past pose sequences but also the agent's interactions with the surrounding environment.

While our work focuses on leveraging text via Knowledge Distillation (KD), we did not explicitly integrate the 3D scene information provided by LiDAR. Including 3D scene data as an additional modality along with human pose, text, and trajectory could further enhance understanding of motion intent and improve predictions of human behavior.

\begin{figure*}
    \includegraphics[width=0.99\textwidth]{figures_supp/sit_viz.PNG} \vspace{-7pt}
    \caption{
    An example scene for SIT dataset. The agent caption $\mathcal{S}_\text{A}$ are acquired from VLM with prompt "What is the person doing?".
    }
    \label{fig:sitViz}
    \vspace{-5pt}
\end{figure*}

\newpage

\begin{figure*}
    \includegraphics[width=0.99\textwidth]{figures_supp/jrdb1.PNG} \vspace{-7pt}
    \caption{
    Example indoor scene from JRDB dataset. Agent caption $\mathcal{S}_\text{A}$ and interaction caption $\mathcal{S}_\text{R}$ are parsed from annotation. Captions of only a few agents are described.
    }
    \label{fig:jrdbViz1}
    \vspace{-5pt}
\end{figure*}

\begin{figure*}
    \includegraphics[width=0.99\textwidth]{figures_supp/jrdb2.PNG} \vspace{-7pt}
    \caption{
    Example outdoor scene from JRDB dataset. Agent caption $\mathcal{S}_\text{A}$ and interaction caption $\mathcal{S}_\text{R}$ are parsed from annotation.
    }
    \label{fig:jrdbViz2}
    \vspace{-5pt}
\end{figure*}

\newpage

\begin{figure*}
    \includegraphics[width=0.99\textwidth]{figures_supp/qual_jrdb.png} \vspace{-7pt}
    \caption{
    Additional qualitative result on JRDB dataset. The left two figures compare prediction result with and without KD on student HiVT model using $\mathcal{X}+\mathcal{P}$ modalities. 
    The right figure compares the effect of using interaction text $\mathcal{S}_\text{R}$ on HiVT model only using $\mathcal{X}$ modality.
    }
    \label{fig:qualJRDB}
    \vspace{-5pt}
\end{figure*}

\begin{figure*}
    \includegraphics[width=0.99\textwidth]{figures_supp/qual_sit.png} \vspace{-7pt}
    \caption{
    Qualitative result on SIT dataset. Agent text captions are acquired from VLM with prompt "What is the person doing?". 
    Prediction results between HiVT models using $\mathcal{X}+\mathcal{P}$ modalities with and without KD are compared. 
    }
    \label{fig:qualSIT}
    \vspace{-5pt}
\end{figure*}
